# Supplementary material for: Switching picosecond magnetoacoustic regimes in a ferromagnetic waveguide
Source: arXiv:2505.09579 ancillary file (2026-07-13)
Supplement: Supplementary file 1 [file Suppl_mat.pdf]

# Three regimes of a picosecond magnetoacoustics in ferromagnetic structures:

## Supplementary Materials

P. I. Gerevenkov,<sup>1,\*</sup> Ia. A. Mogunov,<sup>1</sup> Ia. A. Filatov,<sup>1</sup> N. S. Gusev,<sup>2</sup>  
M. V. Sapozhnikov,<sup>2,3</sup> N. E. Khokhlov,<sup>1</sup> and A. M. Kalashnikova<sup>1</sup>

<sup>1</sup>*Ioffe Institute, St. Petersburg 194021, Russia*

<sup>2</sup>*Institute for Physics of Microstructures,  
RAS, Nizhny Novgorod 603087, Russia*

<sup>3</sup>*Lobachevsky State University of Nizhny Novgorod, Nizhny Novgorod 603022, Russia*

(Dated: June 1, 2025)

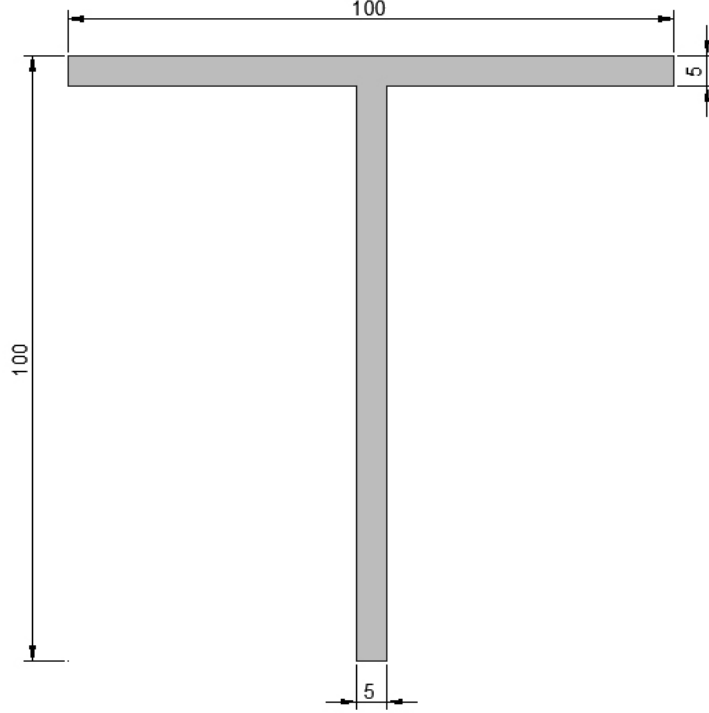

FIG. S.1. **Pattern for the fabrication of T-shaped permalloy structures with dimensions indicated.** Proportions are preserved. Dimensions are given in microns.

## I. SAMPLE PREPARATION DETAILS AND MAGNETIC PARAMETERS MEASUREMENT

T-shaped permalloy structures were fabricated using the lift-off technique. For this purpose, a photoresist mask made of AZ1512 was created on a monocrystalline silicon substrate with a natural oxide layer. Exposure was performed using the Heidelberg Instruments  $\mu$ PG 101 maskless lithography laser writer. The photoresist development was done by MIF726. The pattern used for exposure is shown in Fig. S.1. The silicon substrate was pre-cleaned chemically in an ultrasonic bath successively using toluene, acetone, and isopropyl alcohol for 10 min. The quality of the cleaning was controlled by measuring the surface topography with an atomic force microscope. The root-mean-square (RMS) roughness of the cleaned substrate was found to be no more than 0.4 nm.

Next, the NiFe film with thickness about 20 nm was deposited onto the substrate with the mask using magnetron sputtering. To prevent natural oxidation of the metallic film,

---

\* petr.gerevenkov@mail.ioffe.ru; <http://www.ioffe.ru/ferrolab/>

a 5 nm thick Si layer was deposited on the top. The ferromagnetic film was sputtered at room temperature in an argon atmosphere at  $4 \cdot 10^{-3}$  Torr. The vacuum chamber was pre-pumped down to  $10^{-6}$  Torr. The thicknesses of the metallic layers were controlled by preliminary measurements on test samples using X-ray diffractometry. The sputtering rate of permalloy was  $0.14 \text{ nm s}^{-1}$ . To remove unexposed regions, the sample was placed in a dimethylformamide in ultrasonic bath for 10 min. At the final stage the sample was cleaned by isopropyl alcohol.

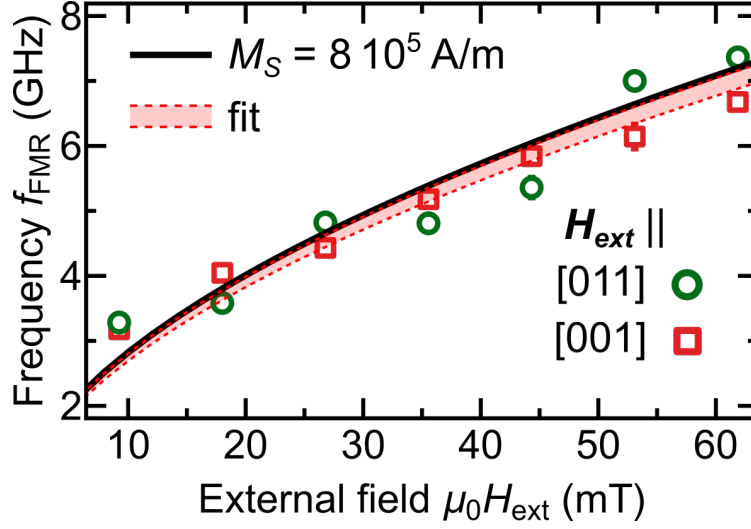

FIG. S.2. **Ferromagnetic resonance frequency vs external magnetic field value.** External field is applied along [011] (green) and [001] (red) crystallographic directions in substrate plane. The red dashed lines and shading show the spread of best fit of the experimental results using Eq. (S.1). Black solid line represent  $f_{\text{FMR}}$  dependence calculated at  $M_S = 8 \times 10^5 \text{ A/m}$ , as used for micromagnetic simulation.

The FMR frequency was measured in continuous film using the pump-probe technique with pump and probe spots coinciding. The frequency was determined from the FFT peak position in the temporal signal of the laser-induced magnetization precession. Measurements with the field applied along different crystallographic directions in the substrate plane do not demonstrate significant differences (see Fig. S.2). Thus, to determine the saturation magnetization, we used Kittel's formula for the case of an isotropic ferromagnetic film:

$$f_{\text{FMR}} = \frac{\mu_0 \gamma}{2\pi} \sqrt{H_{\text{ext}}(H_{\text{ext}} + M_S)}, \quad (\text{S.1})$$

where  $\mu_0 = 4\pi \cdot 10^{-7} \text{ H m}^{-1}$  is magnetic constant,  $\gamma = 1.76 \times 10^{11} \text{ rad s}^{-1} \text{ T}^{-1}$  is gyromagnetic

ratio,  $H_{ext}$  is external magnetic field strength and  $M_S$  is magnetization saturation.

The value, obtained from the best fit using Eq. (S.1) is  $M_S = (7.59 \pm 0.32) 10^5 \text{ A m}^{-1}$ . This value is slightly lower than the literature data [1, 2], which can be attributed to parasitic heating in pump-probe experiments. The ferromagnetic layer and the structure exhibit only shape magnetic anisotropy. In the micromagnetic modeling we used the literature value of  $M_S = 8 \times 10^5 \text{ A m}^{-1}$  [3, 4].

## II. MEASUREMENT TECHNIQUE

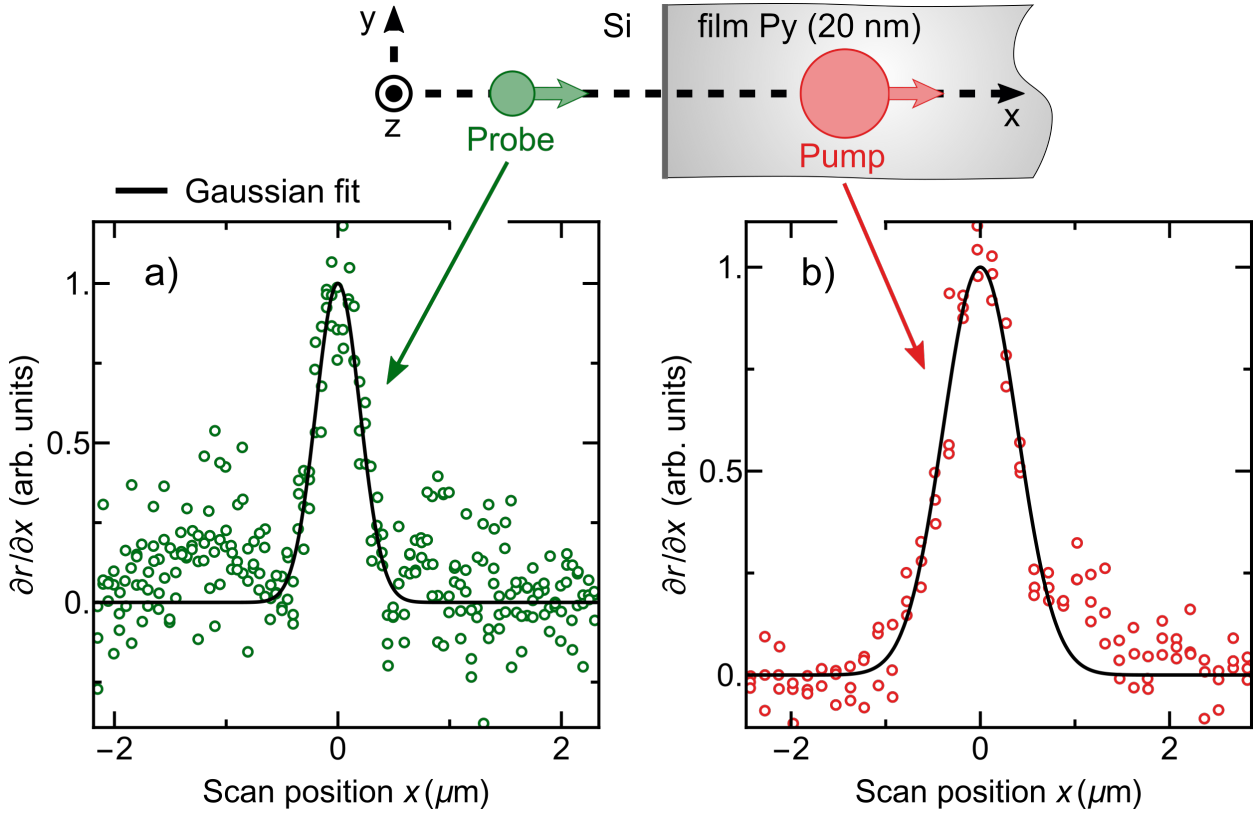

FIG. S.3. **Measurements of the reflectivity change vs. coordinate across the edge.** Reflection change measurements for (a) probe and (b) pump pulses vs. coordinate across the edge. Black solid line shows fit by the Gaussian function.

The pump and probe pulses with duration 120 fs, repetition rate 75 MHz, and central wavelengths 680 nm and 525 nm, respectively, are generated with a femtosecond laser system with tunable wavelength. Linearly polarized pulses are focused on the sample surface normally on the film side using a micro-objective lens into spots with diameters of 0.5 (probe)

and  $0.9\ \mu\text{m}$  (pump). Strongly focused pump and probe spots allow detection of wavepackets over a wide range of wavenumbers  $-2 \div 2\ \mu\text{m}^{-1}$ . The pump pulse fluence is  $4\ \text{mJ}/\text{cm}^2$ . The fluence of the probe pulses is about 20 times lower. Detection is performed using a standard optical balanced circuit using the lock-in detection technique at the pump pulse modulation frequency. The time and space resolution are obtained using an optomechanical delay line and a piezoelectric mirror in the path of the probe pulses, respectively. SAWs are excited with a pump spot placed at the edge of Py film since no generation was observed upon excitation of bare Si substrate. The pump polarization has no effect on the generated waves owing to the thermal excitation mechanism, as discussed in [5–7]. This validates thermal expansion of the film as a SAW excitation mechanism. All measurements were performed at room temperature.

The position in the structure is detected by reflectance measurements ( $r$ ), which differs for the Si substrate and the NiFe film. Fig. S.3 shows the result of  $\partial r/\partial x$  measuring vs. the coordinate  $x$  perpendicular to the edge of the structure. The maximum change in signal corresponds to the edge coordinate ( $x = 0$  on the plots). The fit of the dependences by a Gaussian allows us to estimate the FWHM of the convolution of the pulse spatial profile with the structure edge. The FWHM values of the data in the figure are for probe  $0.47 \pm 0.02\ \mu\text{m}$  (Fig. S.3 a), for pump  $0.92 \pm 0.03\ \mu\text{m}$  (Fig. S.3 a) and vary only slightly with shifts along the edge. In this regard, we assumed the edge of the structure to be sharp and used the measured values as an estimate of the pump and probe areas.

### III. MAGNETOSTATIC WAVE DISPERSIONS SIMULATION

Calculations were performed using the GPU-accelerated micromagnetic framework mumax<sup>3</sup> [4]. We used permalloy magnetic parameters at room temperature with saturation magnetization  $M_S = 8 \times 10^5\ \text{A}/\text{m}$ , an exchange stiffness parameter  $A = 1.3 \times 10^{-11}\ \text{J}/\text{m}$ , and Gilbert damping parameter  $\alpha = 0.01$  [1, 8]. The modeled structure has the same geometry as the experimental one with a thickness  $20\ \text{nm}$  and a waveguide width  $5\ \mu\text{m}$ . The total simulation volume was  $20.48(x) \times 20.48(y) \times 0.02(z)\ \mu\text{m}^3$ . Along the  $y$  direction a periodic boundary conditions have been added. We use a cell size of  $5(x) \times 5(y) \times 10(z)\ \text{nm}^3$ , which is less than the magnetostatic exchange lengths  $\sqrt{2A/(\mu_0 M_S^2)} = 5.7\ \text{nm}$  in the lateral direction. Since higher harmonics across the thickness of the structure are not observed in the experiment

(see Fig. S.2) and do not require an accurate calculation of the corresponding dispersion, we used a  $z$  cell size that exceeded the exchange length to increase the lateral modeling area.

The impact of an optical pulse excitation was modeled by a local change in saturation magnetization, similar to work [9]. Excitation was carried out by an instantaneous change in the  $M_S$  value, followed by an exponential relaxation with a time parameter  $\tau = 300$  ps. In lateral space, excitation takes the form of a two-dimensional Gaussian distribution with a standard deviation of  $0.5 \mu\text{m}$ . To calculate the local dispersion, two simulations were performed: i) the center of the excitation area coincided with the edge of the structure, the dispersion was determined by a short-time 2D FFT with the window center at a distance of  $1 \mu\text{m}$  from the edge and ii) with the window center at a distance of  $6 \mu\text{m}$  from the edge, the center of the excitation area coincided with the window center.

#### IV. SENSITIVITY OF MEASUREMENTS TO VARIOUS (QUASI-)SAW MODES

In our experiments we detected either reflectivity change or polarization rotation change of a linearly polarized probe pulse. Several types of acoustic waves were visible: surface-skimming longitudinal bulk wave (BW), Rayleigh wave (R-SAW) and Love wave (L-SAW). All these waves have  $k_{\text{SAW}}$ -vectors parallel to the sample surface in a direction of scanning which is a high-symmetry crystallographic direction, namely  $[01\bar{1}]$  or  $[100]$ . For cubic Si substrate, SAWs in these directions split into Rayleigh-like and pure Love waves [10]. Here we compare sensitivity of rotation and reflectivity measurements with respect to the mode and probe polarization (see Fig. S.4).

We consider a 20 nm isotropic Py layer on a semi-infinite isotropic Si substrate,  $x$ -axis is parallel to the scan direction and  $k_{\text{SAW}}$ , while  $z$ -axis is along surface normal. We assume plane acoustic waves which is a good approximation at a distance from the point of excitation exceeding several diameters of a probe spot ( $0.5 \mu\text{m}$ ). We follow the analysis for the probe electric field  $E$  described in [11, 12], assuming monochromatic probe with wave vector  $k||z$ , linear response to strain (small strain-induced perturbations of permittivity tensor  $\varepsilon$ ), slow variation of  $\varepsilon$  compared to optical frequency, in-plane homogeneity of the sample within the probe spot at all times and homogeneity along  $y$ -axis (leading to  $\partial/\partial y=0$ ):

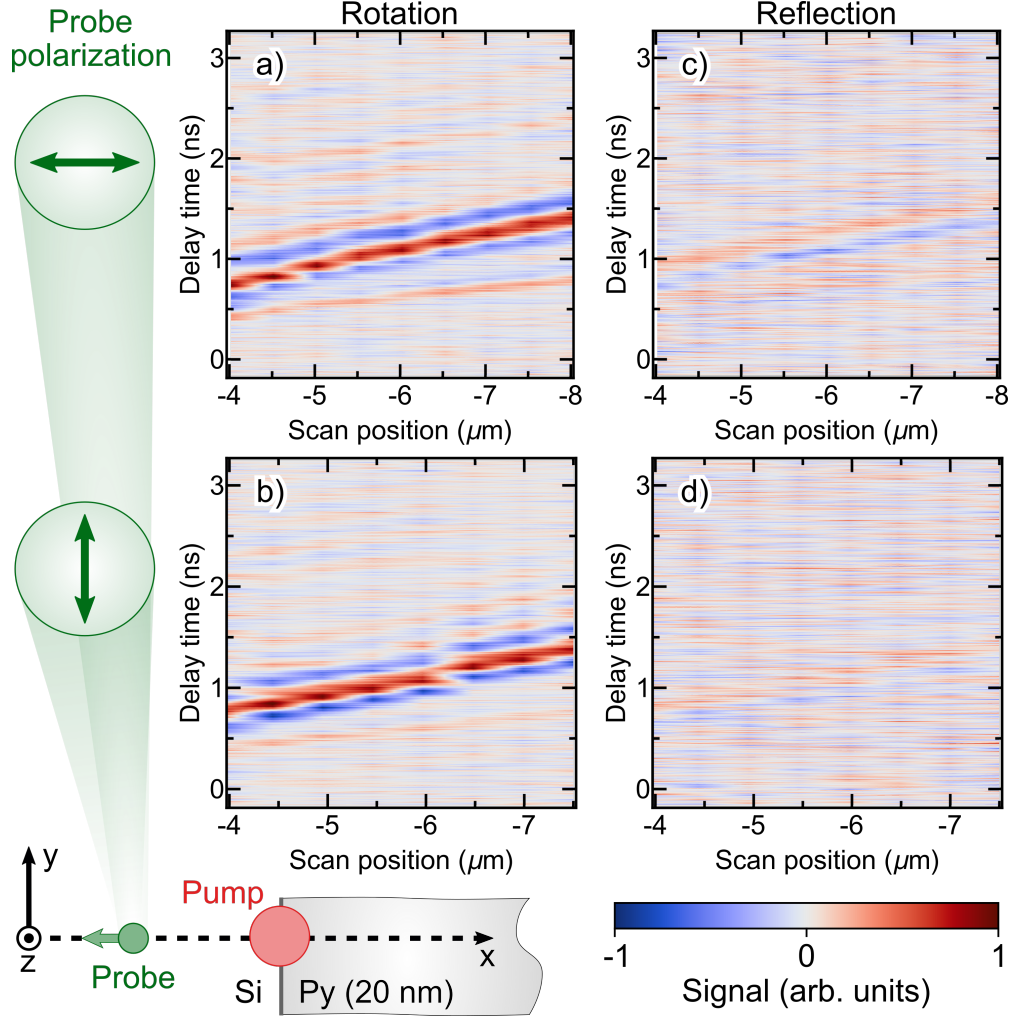

FIG. S.4. **Measurements of the rotation and reflectivity vs. coordinate and time for two orthogonal probe polarizations.** Rotation (a,b) and reflectivity (c,d) vs. coordinate and time maps for probe polarization along (a,c) and across (b,d) BW/SAW propagation direction.

$$E = (e^{ikz} + re^{-ikz}) \begin{pmatrix} E_x \\ E_y \\ 0 \end{pmatrix} + e^{-ikz} \begin{pmatrix} E_x Z_1 + E_y Z_6 \\ E_y Z_2 + E_x Z_6 \\ 0 \end{pmatrix} + 2iku_z r e^{-ikz} \begin{pmatrix} E_x \\ E_y \\ 0 \end{pmatrix}, \quad (\text{S.2})$$

where  $r = \frac{1 - \sqrt{\varepsilon}}{1 + \sqrt{\varepsilon}}$  is a reflection coefficient without strain,  $u_z$  is an atomic displacement at the surface, and  $Z_j$  is described by Eq. (S.3). The first term in Eq. (S.2) is unperturbed reflection, the second is photoelastic effect and the third describes a change in probe light interference due to the surface shift. With an additional assumptions of uniformity of the

strain-induced permittivity tensor modulation  $\varepsilon_{PE}$  within laser penetration depth  $l$  and total absorption within Py layer allowing us to disregard transmission term we write:

$$Z_j \approx -\frac{\varepsilon_{PE,j}}{2ik} \int_l^0 (e^{ikz'} + re^{-ikz'})^2 dz' \quad (\text{S.3})$$

Under these assumptions we can also integrate:  $u_z \approx \eta_3 d$ . From the tensor of photoelastic effect in isotropic case we have [12]:  $\varepsilon_{PE,1} = P_{11}\eta_1 + P_{12}(\eta_2 + \eta_3)$ ,  $\varepsilon_{PE,2} = P_{11}\eta_2 + P_{12}(\eta_3 + \eta_1)$  and  $\varepsilon_{PE,6} = P_{44}\eta_6$  where  $P_{jm}$  and  $\eta_m$  are components of photoelastic tensor and strain tensor, respectively, their indices shown in Voigt notation.

Since we disregard transmission of light into Si substrate, we need only tensor  $\mathbf{P}$  for Py, which is unknown. We use the relation for components of isotropic  $\mathbf{P}$ :  $P_{44} = (P_{11} - P_{12})/2$ . The value of  $P_{12}=1.3-1.2i$  for Nickel is derived from picosecond acoustic experiments [13] for probe wavelength 830 nm. The value of  $P_{44} \approx 0.08-0.04i$  was measured in the work [14] for Cu, which has similar values and signs of real and imaginary parts of  $\varepsilon$  to Py. Finally, the value of unperturbed  $\varepsilon$  at our probe wavelength  $\lambda=525$  nm for Py film was taken from [15] and was used to calculate the penetration depth  $d=11.7$  nm.

For BW, R-SAW and L-SAW the corresponding strain tensors in the chosen coordinate system were used:

$$\eta_{\mathbf{BW}} = \begin{pmatrix} \eta_{BW} \\ 0 \\ 0 \\ 0 \\ 0 \\ 0 \end{pmatrix}; \quad \eta_{\mathbf{R}} = \begin{pmatrix} a\eta_R \\ 0 \\ (1-a)\eta_R \\ 0 \\ \nu\eta_R \\ 0 \end{pmatrix}; \quad \eta_{\mathbf{L}} = \begin{pmatrix} 0 \\ 0 \\ 0 \\ \nu\eta_L \\ 0 \\ \nu\eta_L \end{pmatrix}, \quad (\text{S.4})$$

where  $\nu=0.34$  is the Poisson ratio for Py, calculated from elastic parameters for a thin film [16]. The value  $a=6/7$  illustrates the fact that at the surface of a thin film (thickness  $h$ ,  $k_{SAW}h \ll 1$ ) with Poisson ratio  $\nu=0.34$  the strain of a Rayleigh wave in  $x$  direction is 6 times larger than in  $z$  direction [10]. For calculations we used  $\eta_{BW} = \eta_R = \eta_L = 10^{-4}$ .

Substituting Eqs. (S.4,S.3) into Eq. (S.2) we calculated these values for the change of reflected probe electric field  $\Delta E$  due to the presence of acoustic wave:

$$\begin{aligned}
\Delta E_{BW} &= e^{-ikz} \begin{pmatrix} (-1.26 + 0.69i)10^{-6}E_x \\ (-1.13 + 0.66i)10^{-6}E_y \\ 0 \end{pmatrix}; \\
\Delta E_R &= e^{-ikz} \begin{pmatrix} (0.03 - 2.19i)10^{-6}E_x \\ (0.14 - 2.22i)10^{-6}E_y \\ 0 \end{pmatrix}; \\
\Delta E_L &= e^{-ikz} \begin{pmatrix} (-2.18 + 0.55i)10^{-8}E_y \\ (-2.18 + 0.55i)10^{-8}E_x \\ 0 \end{pmatrix}.
\end{aligned} \tag{S.5}$$

From Eq. (S.5) it is readily seen that for  $x$ - or  $y$ -polarized probe (i.e.  $E_x \neq 0, E_y = 0$  or  $E_x = 0, E_y \neq 0$ ) BW and R-SAW waves yield no contribution to polarization rotation, while L-SAW does. It is also readily seen that optical response to the L-SAW is 2 orders of magnitude lower than for R or BW waves with the same value of strain  $\eta$ . For the reflected intensity  $(\Delta R/R)_j$  ( $j = x, y$  show polarization of incident probe) [11]:

$$\left(\frac{\Delta R}{R}\right)_x = 2\text{Re}\left(\frac{Z_1}{r}\right); \quad \left(\frac{\Delta R}{R}\right)_y = 2\text{Re}\left(\frac{Z_2}{r}\right). \tag{S.6}$$

Here terms quadratic in  $Z_j$  are neglected and an assumption is made that unperturbed sample does not change probe polarization after reflection. For BW  $(\Delta R/R)_{x,BW} = 2.22 \cdot 10^{-6}$ ,  $(\Delta R/R)_{y,BW} = 1.96 \cdot 10^{-6}$ , for R-SAW  $(\Delta R/R)_{x,R} = 2.18 \cdot 10^{-6}$ ,  $(\Delta R/R)_{y,R} = 1.96 \cdot 10^{-6}$ , and for L-SAW both values in Eq (S.6) are zero. We see that L-SAW under our assumptions is not visible in transient reflectivity. For BW and R waves, they are visible in reflectivity change with similar strengths for the same value of strain  $\eta$  and are noticeably ( $\sim 12$  %) different for  $x$ - and  $y$ -polarized incident probe.

If, however, the acoustically unperturbed sample does rotate the polarization plane of reflected probe beam, then both R-SAW and BW would be visible in rotation measurements. This can be seen from the form of elastic contribution to the reflected electric field  $\Delta E_{BW}$  and  $\Delta E_R$  (Eq. S.5). The strain-induced additions to reflected  $x$  and  $y$  polarizations are proportional to *incident*  $E_x$  and  $E_y$ , respectively, therefore if unperturbed reflected polarization rotates, these additions would cause an additional rotation with respect to the new, rotated, state of polarization.

As shown in the main text, the additional contribution to the detection of acoustic wavepacket in Py film comes from the magneto-optical polar Kerr effect. However, for detection in the Si substrate, we also observe a signal from the BW and R-SAW in both, the rotation and reflection measurements. The intensity of the reflection signal changes when the polarization plane is rotated by 90 degrees (from  $||x$  to  $||y$ ), as can be seen in Fig. S.4 c,d. This fact coincides with the model described previously. We attribute the presence of a signal in the case of the polarization plane rotation measurement to the non-zero rotation of reflected probe polarization in the absence of acoustic waves, as described above, and to a non-zero  $x(y)$  component of the nominally  $y-(x-)$ polarized probe pulse in a real experiment. Due to a high sensitivity of our rotation measurements (compared to reflectivity ones, see Section VIII) we therefore can observe a signal from BW and R-SAW (see the Fig. S.4 a,b).

## V. DISPERSION RELATIONS OF SAW WAVES

Here we describe calculations of dispersion relations for quasi-Rayleigh (R-SAW) and Love (L-SAW) modes in a system "isotropic Py layer on a semi-infinite isotropic Si substrate". The stiffness tensor for Py was taken from ref. [16], where it was evaluated for a thin isotropic Py film. The isotropic tensor for Si approximating the real one [17] was calculated using procedure described in [18]. We calculated SAW modes separately for Love and for Rayleigh, Sezawa waves implementing a well-known formalism (see, e.g. [10, 19]) using custom MATLAB codes. The results are summarized on Figure S.5.

Note that for the used thickness of Py  $d=20$  nm and laser generated  $k_{SAW}$ -vectors  $\lesssim 2 \mu m^{-1}$  no Sezawa or higher orders Love modes can propagate (see Fig. S.5(2)) leaving only 3 possible waves: two SAWs (R and L) and a surface-skimming longitudinal bulk wave (BW). This is also true for a real cubic Si substrate in a case of the propagation along a high-symmetry direction  $[01\bar{1}]$  or  $[100]$  [10] which is indeed the case in our experiments. For such a thin film the velocity of R-SAW is close to Rayleigh sound velocity in isotropic Si  $v_{R,Si}=4.95$  km/s, while the L-SAW is close to a transverse acoustic bulk wave (TA) in Si with velocity  $v_{TA,Si}=5.40$  km/s [17], and therefore L-SAW is faster than R-SAW wave (see Fig. S.5(1)).

From the experiments we obtain for pure Si substrate in the  $[100]$  direction  $v_{BW,Si}=9.10 \pm$

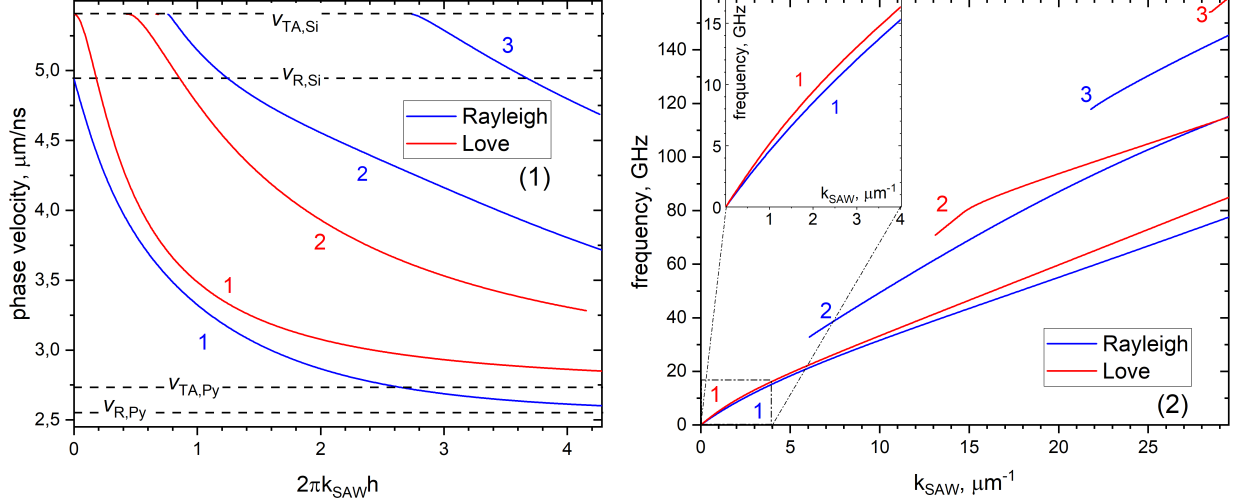

FIG. S.5. Calculation results for SAWs in Py/Si system (isotropic parameters). Numbers 1-2-3 indicate the order of the modes (blue for Rayleigh and Sezawa, red for Love). (1) phase velocities vs dimensionless wave vector  $k_{\text{SAW}}h$ , where  $h=20$  nm is Py film thickness. (2) dispersion relation frequency  $f$  vs wave vector  $k_{\text{SAW}}$ . The inset enlarges the  $k_{\text{SAW}}$ -range accessible in our experiments.

0.25 km/s,  $v_{\text{SAW,Si}}=4.82 \pm 0.03$  km/s, and in the  $[01\bar{1}]$  direction  $v_{\text{BW,Si}}=10.25 \pm 0.15$  km/s,  $v_{\text{SAW,Si}}=6.03 \pm 0.04$  km/s. For Py film on Si substrate in the  $[011]$  direction we obtain  $v_{\text{BW,Py}}=9.8 \pm 0.1$  km/s,  $v_{\text{R-SAW,Py}}=4.04 \pm 0.02$  km/s, and  $v_{\text{L-SAW,Py}}=5.42 \pm 0.03$  km/s.

## VI. MOVING PULSE EXCITATION MODEL

To reveal criteria for transition between Cherenkov-like MSW, ME wave and non-resonant regimes, we employ theoretical analysis where the acoustic wave packet is approximated by an effective field perturbation via magnetoelastic coupling. The torque moves at a speed  $v$  through a medium with a spin-wave dispersion  $f(k)$ . The model does not take into account the influence of the excited magnetization dynamics on the exciting wavepacket. Then the spatial distribution of magnetization dynamics ( $m$  component) can be evaluated as [7, 20, 21]:

$$m(x) = \int_{-\infty}^0 dt \int_{-\infty}^{\infty} dk \mathcal{F}[T(x - vt)] e^{-2\pi i [f(k)(1-i\alpha)t - kx]}, \quad (\text{S.7})$$

Gilbert damping introduced as an imaginary part of the frequency with parameter  $\alpha$ . The operator  $\mathcal{F}(T(x))$  denotes the Fourier transform of the LL-torque profile.

To perform the integration of Eq. (S.11) in a vicinity of a point  $k_c$  where dispersions for

magnetostatic and ascoustic waves are tangent, let us start with temporal integral. Using a moving coordinate system  $\tilde{x} = x - vt$  we obtain:

$$\int_{-\infty}^0 \mathcal{F}(T(\tilde{x})) e^{-2\pi i(f(k)(1-\imath\alpha)t - k(\tilde{x}+vt))} dt = -\frac{1}{2\pi} \frac{\imath e^{2\pi i k \tilde{x}}}{kv - f(k)(1-\imath\alpha)}, \quad (\text{S.8})$$

Next, to integrate over  $k$ , we need to specify an explicit form of dispersion. To do this, we perform the expansion  $f(k) \approx f(k_c) + f'(k_c)(k - k_c) + 0.5f''(k_c)(k - k_c)^2$  near the point of intersection with the tangent  $v_c k$  and use condition  $f'(k_c) = f(k_c)/k_c = v_c$  (here  $f'(k_c)$  is  $df(k)/dk|_{k=k_c}$ ). Thus, we obtain a quadratic dependence on  $k$  in the denominator of Eq. (S.8). We perform the expansion by roots:

$$k_{1,2} = k_c \left( \Xi(v_n) \pm \sqrt{\Xi(v_n)^2 - 1} \right), \quad (\text{S.9})$$

$$\Xi(v_n) = v_n \frac{1 + \imath\alpha}{1 + \alpha^2} - v_{nc} + 1, \quad v_n = \frac{v}{k_c f''(k_c)}, \quad v_{nc} = \frac{v_c}{k_c f''(k_c)}$$

Now the integral Eq. (2) with Eq. (S.8,S.9) is by definition the inverse Fourier transform of the functions product, which allows us to use the convolution theorem:

$$m(\tilde{x}) = -\frac{\imath}{2\pi} \int_{-\infty}^{\infty} \mathcal{F}(T(\tilde{x})) \frac{e^{2\pi i k \tilde{x}}}{(k - k_1)(k - k_2)} dk = -\frac{\imath}{2\pi} \mathcal{F}^{-1} \left( \frac{\mathcal{F}(T(\tilde{x}))}{(k - k_1)(k - k_2)} \right) = \quad (\text{S.10})$$

$$= -\frac{\imath}{2\pi} \mathcal{F}^{-1}(\mathcal{F}(T(\tilde{x}))) * \mathcal{F}^{-1}((k - k_1)^{-1}(k - k_2)^{-1}),$$

For the profile of the exciting pulse, up to normalization, we obtain  $\mathcal{F}^{-1}(\mathcal{F}(T(\tilde{x}))) = T(\tilde{x})$ . The inverse Fourier transform of the second function:

$$\mathcal{F}^{-1}((k - k_1)^{-1}(k - k_2)^{-1}) = \frac{2\pi\imath}{k_1 - k_2} \{ e^{2\pi i k_1 \tilde{x}} \Theta[\tilde{x} S_{\Im}(k_1)] S_{\Im}(k_1) - e^{2\pi i k_2 \tilde{x}} \Theta[\tilde{x} S_{\Im}(k_2)] S_{\Im}(k_2) \}, \quad (\text{S.11})$$

which leads us to the Eq. (1) in the main text. Although the analytical expression is obtained in the vicinity of tangential point of two dispersions, the drawn conclusions are valid across wide wavevectors range.

## VII. PHASE VELOCITY MEASUREMENTS

Since the profile of the acoustic packet does not change during propagation, the phase positions in Fig. S.6 a correspond to the minimum/maximum lines of the signal  $(s(t, x))$ . To isolate a specific phase, we used a Gaussian window of weighting coefficients  $G(t, x, v, x_0)$  (see Fig. S.6 b).

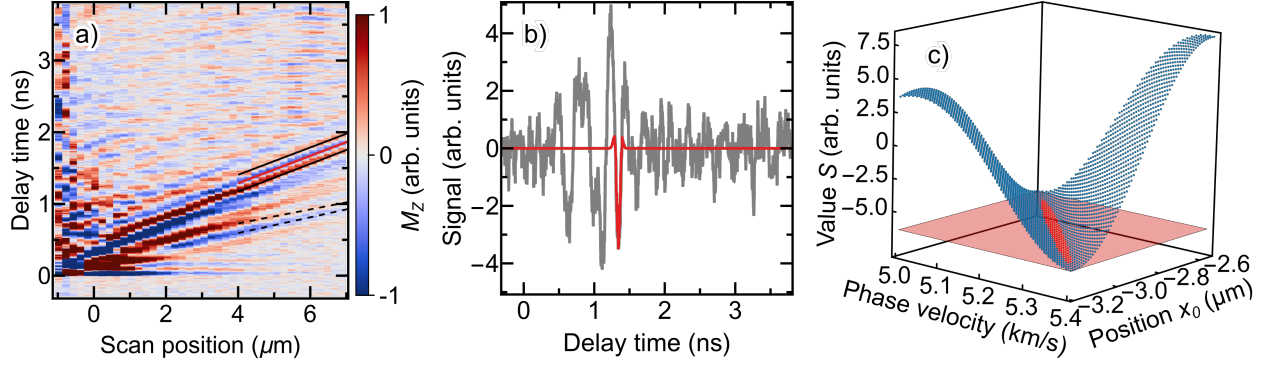

FIG. S.6. **Phase velocity measurements method.** (a) Maps of probe polarization rotation vs. distance and delay time between excitation and detection for external magnetic field  $\mu_0 H_{ext} = 66$  mT along the propagation direction. Different phases of propagating acoustic packets are highlighted by lines. (b) Example of pump-probe signal (gray) and  $s(t, x)G(t, x, v, x_0)$  (red) from (a) at  $x = 4 \mu\text{m}$  vs delay time. (c)  $S(v, x_0)$  values vs  $v$  and  $x_0$  (blue) and  $S(v, x_0) \leq 0.99 S_{min}$  (red).  $S_{min}$  is shown by red plane. Best fit isophase line is shown in (a) in red.

The total value  $S(v, x_0)$  with Gaussian weighting factors defined as:

$$S(v, x_0) = \sum_x \sum_t s(t, x) G(t, x, v, x_0) \quad (\text{S.12})$$

$$G(t, x, v, x_0) = \exp \left( -\frac{(t - v^{-1}(x - x_0))^2}{2\sigma^2} \right),$$

where  $s(t, x)$  – pump-probe signal measured at delay time  $t$  and position  $x$ ,  $v$  and  $x_0$  are velocity and phase position at  $t = 0$  variables,  $\sigma$  is a standard deviation of weighting factors, which is used  $= 1/30$  ns (example of  $s(t, x)G(t, x, v, x_0)$  is shown in Fig. S.6 b by red curve).

The minimum/maximum of  $S(v, x_0)$  in the  $v, x_0$  coordinates corresponds to the best fit of the phase. The average values of the  $v$  set, corresponding to 1-0.99 of the minimum/-maximum of  $S(v, x_0)$ , were used as the phase velocity values (red points in Fig. S.6 c). The errors in the velocity plots in the main text correspond to the standard deviation of this set of points.

## VIII. SIMULTANEOUS ROTATION AND REFLECTION MEASUREMENTS

For the number of signal vs distance and delay time maps, the transient change of reflectivity was measured simultaneously with the rotation of the polarization plane. The

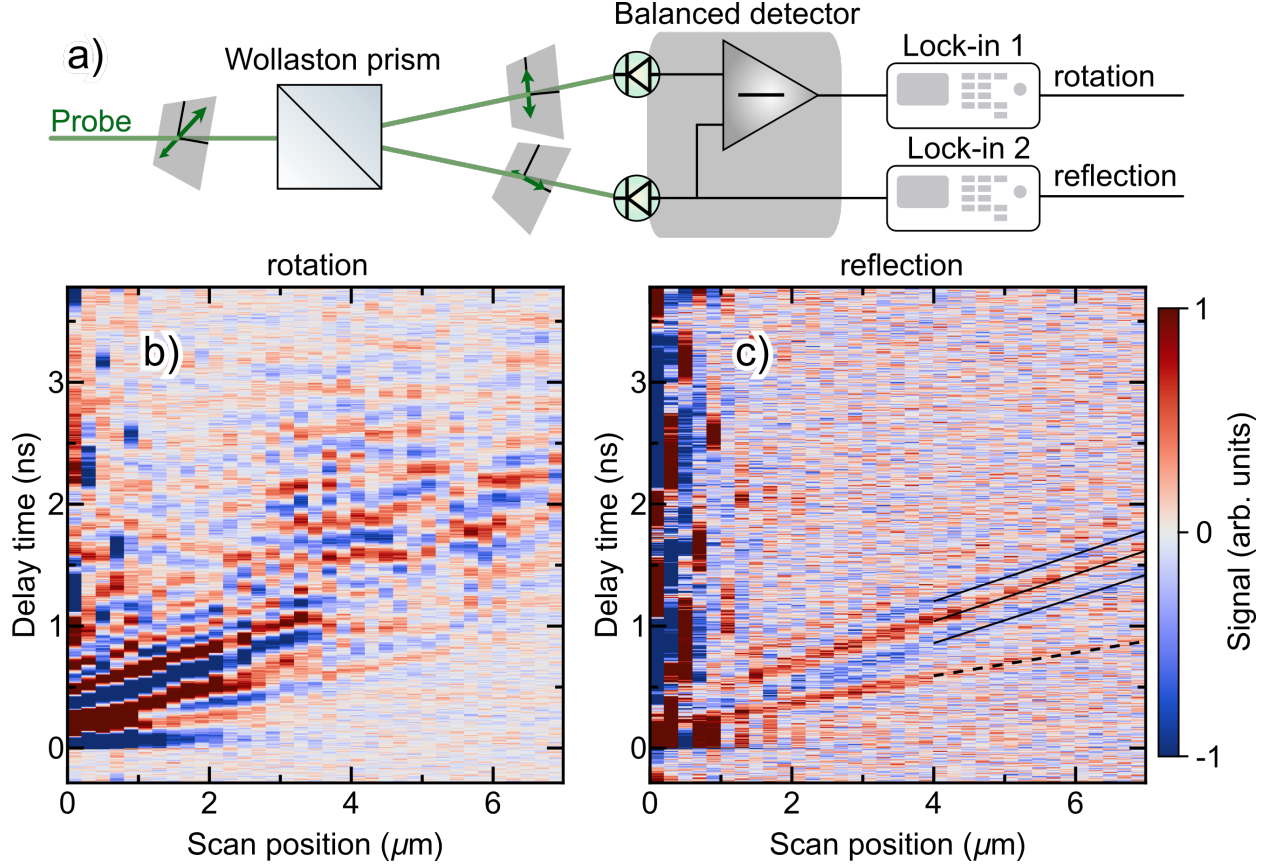

FIG. S.7. **Simultaneous measurements of polarization plane rotation and reflection.**

(a) Detection scheme. Signal maps of pump induced polarization plane rotation (b) and reflection (c) vs distance and delay time between excitation and detection. Measurements were carried out at  $\mu_0 H_{ext} = 5 \text{ mT}$  in the BVSW geometry.

detection scheme is shown in Fig. S.7 a. The Wollaston prism splits the probe pulse reflected from the sample into two orthogonal polarizations. The polarization plane before the prism was rotated using a half-wave plate so that in the absence of a magneto-optical response the intensities of the pulses after the prism were equal. To measure the polarization rotation, the intensity difference was detected, the signal of which, after amplification, was directed to Lock-in 1. To measure the reflection, the unamplified signal from one of the diodes was directed to Lock-in 2, the signal of which, in the approximation of small polarization rotations, corresponds to half reflection change. Both lock-ins detect signals at the pump pulses modulation frequency.

Figure S.7 b shows a map of the magneto-optical signal similar to that shown in Fig. 3 b of the main text. Figure S.7 c shows a map of the reflection signal measured simultaneously

with the rotation signal (Fig. S.7 b). The lines in Fig. S.7 c show the isophase lines used to estimate the velocity of the acoustic packets (see the filling points in Fig. 3 k of the main text).

## IX. DEPENDENCE OF THE ME PHASE VELOCITY ON THE EXTERNAL MAGNETIC FIELD MAGNITUDE

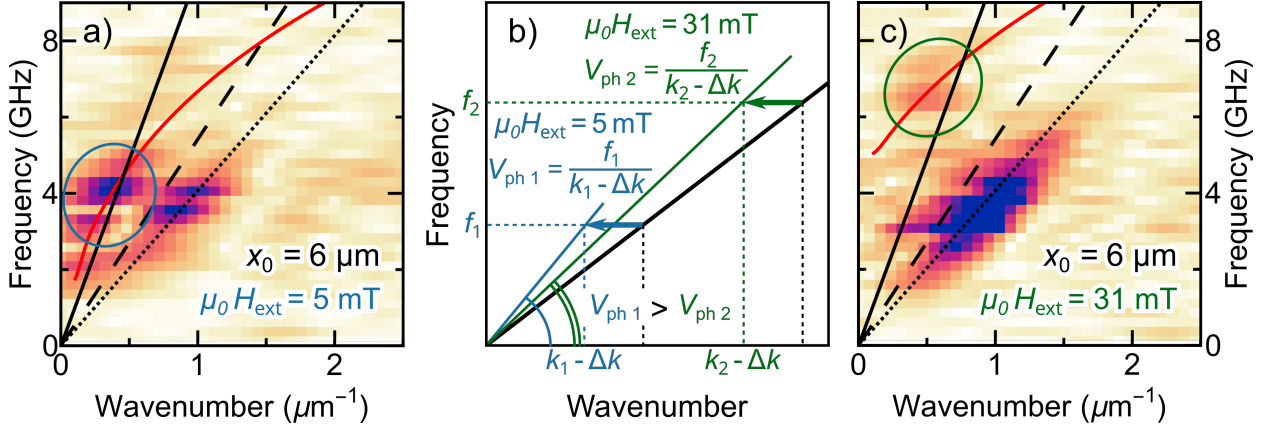

FIG. S.8. **Effect of the BW-MSW hybridization on the phase velocity of the wavepacket.** (a, c) Short-time 2D FFT, centered at  $6 \mu\text{m}$  from the excitation area, of the pump-probe signal in an external magnetic field of 5 (a) and 31 (c) mT, respectively. Measurements are performed in  $\mathbf{H}_{\text{ext}} \parallel \mathbf{k}$  geometry. The black lines show the dispersions of the BW, L-, and R-SAW (solid, dashed, and dotted lines, respectively). The red line shows the dispersion of the MSW obtained from the micromagnetic simulation. (b) Scheme of the effect of the dispersion deviation from the linear law for the different external magnetic field values on the phase velocity magnitude.

Hybridization of the BW with the MSSW leads to a deviation of the resulting dispersion from the linear dependence. Experimentally, we observe a shift in the dispersion towards the smaller  $k$  in the vicinity of the intersection point (see Fig. S.8 a and c). This shift leads to an increase in the phase velocity  $v_{\text{ph}} = \frac{f}{k - \Delta k}$  due to a decrease in the denominator. Assuming that the shift  $\Delta k$  is independent of  $H_{\text{ext}}$ , an increase in the frequency of the intersection point with increasing external magnetic field value leads to a decrease in the phase velocity of the ME wavepacket, as shown in the Fig. S.8 b.

The dispersion dependence of hybridized magnetostatic and acoustic wave can be de-

scribed as [22]:

$$(f^2 - f_{MSW}(k)^2) (f^2 - f_{SAW}(k)^2) - f_{int}^4 = 0, \quad (\text{S.13})$$

where  $f$  is a variable parameter,  $f_{MSW}$  is the frequency of the magnetostatic wave,  $f_{SAW}$  is the frequency of the acoustic wave,  $f_{int}$  is a parameter describing the interaction between two waves and  $k$  is the wave vector.

- 
- [1] Y. Zhao, Q. Song, S.-H. Yang, T. Su, W. Yuan, S. S. P. Parkin, J. Shi, and W. Han, Experimental investigation of temperature-dependent gilbert damping in permalloy thin films, *Sci. Rep.* **6**, 22890 (2016).
  - [2] L. C. C. M. Nagamine, J. Geshev, T. Menegotto, A. A. R. Fernandes, A. Biondo, and E. B. Saitovitch, Ferromagnetic resonance and magnetization studies in exchange-coupled NiFe/Cu/NiFe structures, *Journal of magnetism and magnetic materials* **288**, 205 (2005).
  - [3] N. Khokhlov, A. Khramova, I. A. Filatov, P. Gerevenkov, B. Klinskaya, and A. Kalashnikova, Néel domain wall as a tunable filter for optically excited magnetostatic waves, *Journal of Magnetism and Magnetic Materials* **534**, 168018 (2021).
  - [4] A. Vansteenkiste, J. Leliaert, M. Dvornik, M. Helsen, F. Garcia-Sanchez, and B. Van Waeyenberge, The design and verification of mumax3, *AIP advances* **4**, 107133 (2014).
  - [5] V. N. Kats, T. L. Linnik, A. S. Salasyuk, A. W. Rushforth, M. Wang, P. Wadley, A. V. Akimov, S. A. Cavill, V. Holy, A. M. Kalashnikova, and A. V. Scherbakov, Ultrafast changes of magnetic anisotropy driven by laser-generated coherent and noncoherent phonons in metallic films, *Phys. Rev. B* **93**, 214422 (2016).
  - [6] L. A. Shelukhin, V. V. Pavlov, P. A. Usachev, P. Y. Shamray, R. V. Pisarev, and A. M. Kalashnikova, Ultrafast laser-induced changes of the magnetic anisotropy in a low-symmetry iron garnet film, *Physical Review B* **97**, 014422 (2018).
  - [7] N. E. Khokhlov, P. I. Gerevenkov, L. A. Shelukhin, A. V. Azovtsev, N. A. Pertsev, M. Wang, A. W. Rushforth, A. V. Scherbakov, and A. M. Kalashnikova, Optical excitation of propagating magnetostatic waves in an epitaxial galfenol film by ultrafast magnetic anisotropy change, *Physical Review Applied* **12**, 044044 (2019).
  - [8] D.-S. Han, S.-K. Kim, J.-Y. Lee, S. J. Hermsdoerfer, H. Schultheiss, B. Leven, and B. Hille-

- brands, Magnetic domain-wall motion by propagating spin waves, *Appl. Phys. Lett.* **94**, 112502 (2009).
- [9] P. I. Gerevenkov, I. A. Filatov, A. M. Kalashnikova, and N. E. Khokhlov, Unidirectional propagation of spin waves excited by femtosecond laser pulses in a planar waveguide, *Physical Review Applied* **19**, 024062 (2023).
  - [10] I. Viktorov, *Rayleigh and Lamb Waves: Physical Theory and Applications*, Ultrasonic Technology (Springer US, 2013).
  - [11] T. Saito, O. Matsuda, M. Tomoda, and O. B. Wright, Imaging gigahertz surface acoustic waves through the photoelastic effect, *J. Opt. Soc. Am. B* **27**, 2632 (2010).
  - [12] O. Matsuda, O. B. Wright, D. H. Hurley, V. Gusev, and K. Shimizu, Coherent shear phonon generation and detection with picosecond laser acoustics, *Phys. Rev. B* **77**, 224110 (2008).
  - [13] T. Saito, O. Matsuda, and O. B. Wright, Picosecond acoustic phonon pulse generation in nickel and chromium, *Phys. Rev. B* **67**, 205421 (2003).
  - [14] K. Pedersen and O. Keller, Photoelastic properties of metals measured by off-null ellipsometry, *Appl. Opt.* **25**, 226 (1986).
  - [15] K. K. Tikuišis, L. Beran, P. Cejpek, K. Uhlířová, J. Hamrle, M. Vaňatka, M. Urbánek, and M. Veis, Optical and magneto-optical properties of permalloy thin films in 0.7–6.4eV photon energy range, *Materials & Design* **114**, 31 (2017).
  - [16] C. Rossignol, B. Perrin, B. Bonello, P. Djemia, P. Moch, and H. Hurdequint, Elastic properties of ultrathin permalloy/alumina multilayer films using picosecond ultrasonics and brillouin light scattering, *Phys. Rev. B* **70**, 094102 (2004).
  - [17] H. J. McSkimin, Measurement of elastic constants at low temperatures by means of ultrasonic waves—data for silicon and germanium single crystals, and for fused silica, *Journal of Applied Physics* **24**, 988 (1953).
  - [18] F. I. Fedorov, *Theory of Elastic Waves in Crystals* (Springer New York, 1968).
  - [19] G. Farnell and E. Adler, 2 - elastic wave propagation in thin layers, in *Physical Acoustics Principles and Methods*, Physical Acoustics, Vol. 9, edited by W. P. Mason and R. N. Thurston (Academic Press, 1972) pp. 35–127.
  - [20] Y. Hashimoto, S. Daimon, R. Iguchi, Y. Oikawa, K. Shen, K. Sato, D. Bossini, Y. Tabuchi, T. Satoh, B. Hillebrands, *et al.*, All-optical observation and reconstruction of spin wave dispersion, *Nature communications* **8**, 15859 (2017).

- [21] M. Yan, A. Kakay, C. Andreas, and R. Hertel, Spin-cherenkov effect and magnonic mach cones, *Physical Review B* **88**, 220412 (2013).
- [22] C. Berk, M. Jaris, W. Yang, S. Dhuey, S. Cabrini, and H. Schmidt, Strongly coupled magnon–phonon dynamics in a single nanomagnet, *Nature communications* **10**, 2652 (2019).
